# Supplementary material for: Visual definition of procedures for automatic virtual scene generation
Source: arXiv:1202.2868 source file (2012-02-10)
Supplement: Supplementary file 1 [file appendix.tex]

% this file is called up by thesis.tex
% content in this file will be fed into the main document

%: ----------------------- name of chapter  -------------------------
\chapter{In-depth analysis of the setup and usage of libprocedural} % top level followed by section, subsection
\label{sec:appendix.libprocedural}

%: ----------------------- paths to graphics ------------------------

% change according to folder and file names
% \ifpdf
%     \graphicspath{{5/figures/PNG/}{5/figures/PDF/}{5/figures/}}
% \else
%     \graphicspath{{5/figures/EPS/}{5/figures/}}
% \fi

%: ----------------------- contents from here ------------------------

This part gives a more in-depth description of how to set up and run libprocedural with another application.
% ---------------------------------------------------------------------------
%: ----------------------- end of thesis sub-document ------------------------
% ---------------------------------------------------------------------------
